# Supplementary material for: Distributed model order reduction of a model for microtubule-based cell polarization using HAPOD
Source: arXiv:2111.00129 source file (2021-10-30)
Supplement: Supplementary file 1 [file appendix.tex]

\section{Appendix}
TODO
